# Supplementary material for: Quantifying Cybersecurity Effectiveness of Dynamic Network Diversity
Source: arXiv:2112.07826 source file (2021-12-15)
Supplement: Supplementary file 1 [file appendix.tex]

\section{Supplementary material}
\subsection{Pseudo-code of Our Algorithm for Initial Diversity Configuration}

Algorithm \ref{alg:assginment} presents the pseudo code for the initial employment of network diversity.
At a high level, the algorithm has three steps: (i) {\em ordering} the nodes according to their degrees to identify the large-degree nodes, which is achieved by function $\textsc{ordering}$ (Lines 12-14); (ii) {\em coloring} the nodes such that large-degree nodes are preferentially assigned with different implementations to reduce defective edges between them, which is achieved by function $\textsc{coloring}$ (Lines 15-28); and (iii) {\em switching} colors of some nodes to decrease the number of defective edges if possible, which is achieved by function $\textsc{switching}$ (Lines 29-33).
%\footnote{move this paragraph there; describing the functionalities of the functions called in the algorithm}

\begin{algorithm}[!htbp]
\algrenewcommand\algorithmicindent{.75em}
\caption{Diversified software stack assignment} \label{alg:assginment}
    \hspace*{\algorithmicindent} \textbf{Input:} $G = (V,E)$ with $n$ computers, $\SW$, $X$ \\ %{\color{blue}the number $y$ of different types of applications}\\
    \hspace*{\algorithmicindent} \textbf{Output:} {$C_0:V\to \SW$}
    \begin{algorithmic}[1]
  \State $Y$ $\gets$ number of different types of applications in $G$
%\State assign application programs to run in each computer 
    \State $V_{\app_{j}} \gets \{\app_{1,j},\ldots,\app_{n,j}\}$ where 
    $1\leq j \leq Y$
    \State $V_{\os} \gets \{\os_{1},\ldots,\os_{n}\}$
    \For{$1\leq j \leq Y$}
    \State $\textsc{ordering}(V_{\app_{j}})$
    \State $\textsc{coloring}(V_{\app_{j}})$
    \State $\textsc{switching}(V_{\app_{j}})$
    \EndFor
    \State $\textsc{ordering}(V_{\os})$
    \State $\textsc{coloring}(V_{\os})$
    \State $\textsc{switching}(V_{\os})$    
    \Procedure{ordering}{$V^{'}$} \Comment{$V^{'}$ is a node set}
    \State Sort $V^{'}$ based on their degree in the descending order
    \EndProcedure
    \Procedure{coloring}{$V^{'}$} 
    \State{Label the implementations from 1 to $X$ }
    \For{$v^{'} \in V^{'}$}
    \State {fetch an implementation from $\SW$ in turn and pre-assign it to node $v^{'}$}
    \If{no defective edges linked to $v^{'}$}
    \State{approve the pre-assignment}
    \Else
    \State{find out some other implementation that does not lead to local defective edges and assign it $v^{'}$
    }
    \If{no applicable implementation}   
    \State {choose the implementation that leads to minimum local defective edges, if more than one candidate exists, choose the implementation that is the same as that of the adjacent node with the lowest degree}
    \EndIf    
    \EndIf
    \EndFor
    \EndProcedure    
    \Procedure{switching}{$V^{'}$}     
    \State {switch the implementation of $v^{'} \in V^{'}$ to another iteratively if that can lead to less defective edges}
    \EndProcedure     
    %\State {\color{red}for each application, sort the nodes according to their degree in the descending order --- what is there are inter-app communications, why not consider all nodes together? need to justify ... write the algorithm at this level of abstraction would make it much easier to understand}
    \end{algorithmic}
\end{algorithm}
